# Supplementary material for: Towards providing reliable job completion time predictions using PCS
Source: arXiv:2401.10354 source file (2024-01-18)
Supplement: Supplementary file 1 [file appendix.tex]

\section*{APPENDIX}
\setcounter{section}{0}
\section{Sensitivity of discovered configs}
\begin{figure}
    \centering
    \includegraphics[width=\columnwidth]{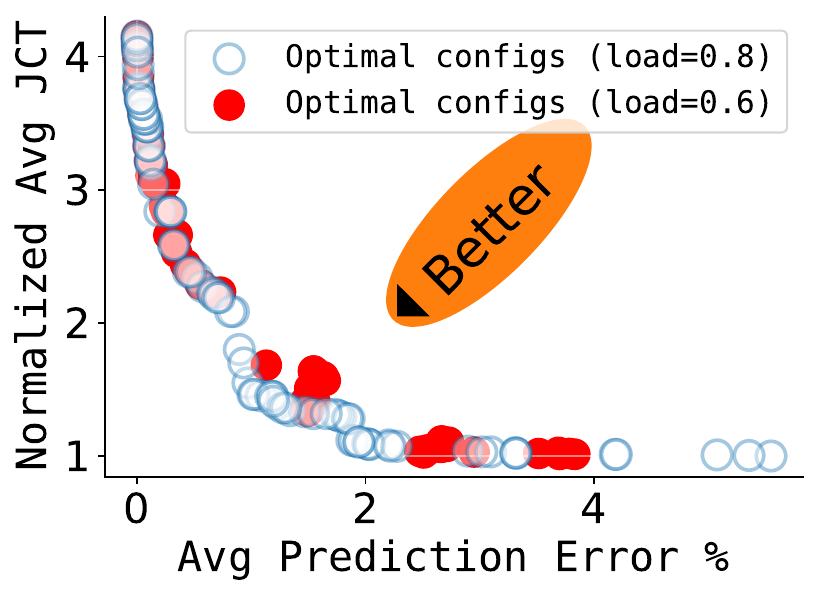}
    \caption{Sensitivity of configs to workload.}
    \label{fig:sensitivity}
\end{figure}
Each configuration is discovered based on simulations of a particular workload. To evaluate the sensitivity of these configs to the specific workload, we evaluate configurations generated for a workload at 60\% load when running in a system at 80\% load. This demonstrates how \sys{} performs when the initial simulation is an estimate of the jobs \sys{} will receive, but not an exact match. Fig~\ref{fig:sensitivity} shows the Pareto points of optimal configs for the 80\% workload, along with the configs that would be optimal for a 60\% workload. The difference between these points are small, with greater than 75\% of the configurations being less than 10\% away from an optimal point in both dimensions. This demonstrates the robustness of configurations to varying load conditions.
